# Supplementary material for: Fundamental precision bounds for three-dimensional optical localization microscopy with Poisson statistics
Source: arXiv:1803.01776 ancillary file (2018-03-06)
Supplement: Supplementary file 1 [file supplemental-material-1.pdf]

# Supplemental Material

## Fundamental precision bounds for three-dimensional optical localization microscopy with Poisson statistics

Mikael P. Backlund, Yoav Shechtman, Ronald L. Walsworth

# I. ADDITIONAL FIGURES

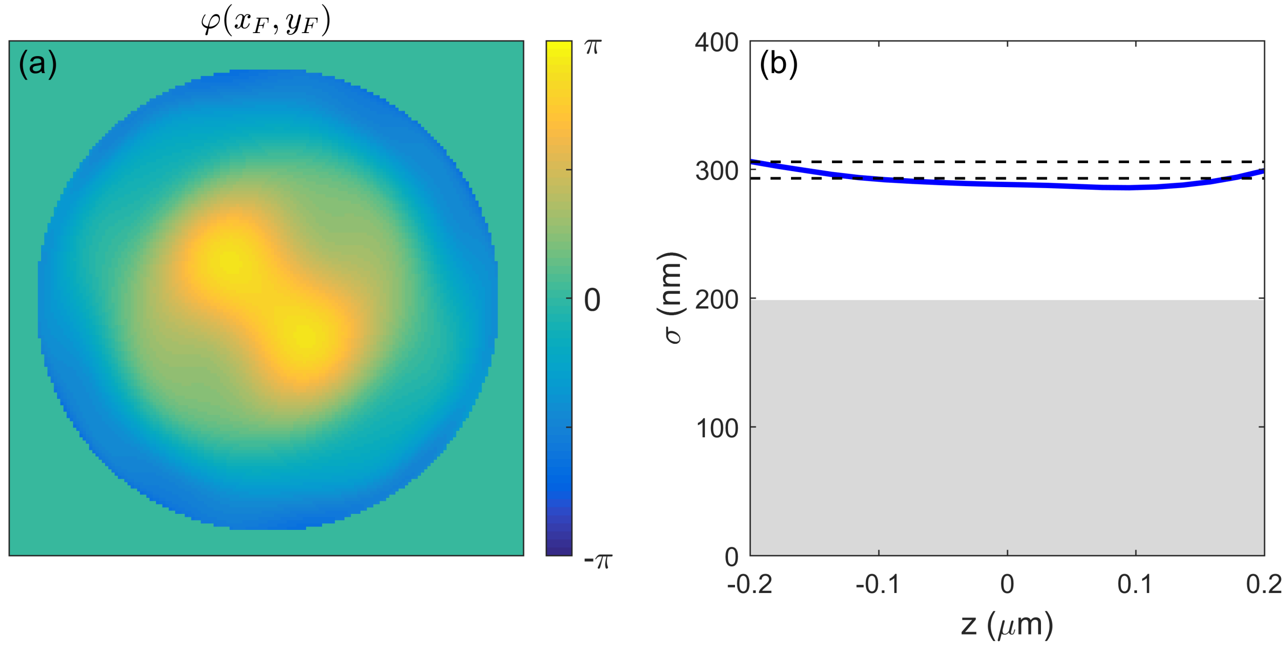


FIG. S1. Results of PSF optimization by minimization of $\sigma_z^{(\mathrm{CRB})}$. We employed the same basic algorithm as was used previously to produce the Saddle-Point [1] and Tetrapod [2] family of PSFs. Key differences here are that we assume zero background light and we proceed via minimization of the average value of $\sigma_z^{(\mathrm{CRB})}$ over a specified range in $z$, rather than minimizing $\sqrt{\left(\sigma_x^{(\mathrm{CRB})}\right)^2 + \left(\sigma_y^{(\mathrm{CRB})}\right)^2 + \left(\sigma_z^{(\mathrm{CRB})}\right)^2}$. We choose a relatively narrow range in $z$ of 400 nm in order to push toward optimal local CRB, as there is known to be a tradeoff between $z$ range and precision [2]. For consistency here we assume NA = 1.4, $\lambda_\circ = 670$ nm, and matched immersion index of $n = 1.518$. (a) Phase mask $\varphi(x_F, y_F)$ resulting from optimization. (b) Photon-normalized CRB for $z$ precision of optimized PSF (blue line). Gray box shows QCRB. Lower dashed black line is the minimum CRB for $z$ estimation of the standard PSF, while upper dashed black line is the minimum CRB for $z$ estimation of an astigmatic PSF with strength $A_{\mathrm{astig.}} = 1$ (see Fig. S2).

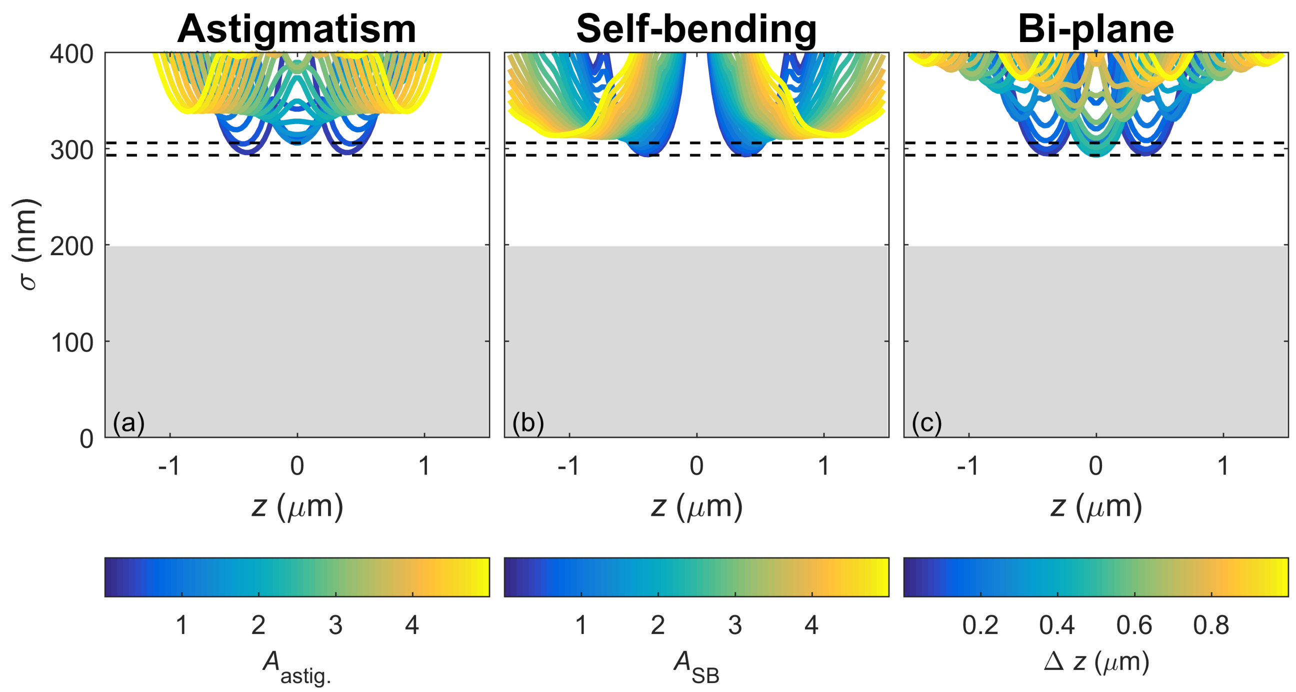


FIG. S2. Comparison of photon-normalized QCRB for single-objective $z$ precision (gray boxes) to the CRBs obtained by several types of engineered microscopes. In each panel the lower dashed black line is the minimum CRB obtained by the standard PSF, while the upper dashed black line is the minimum CRB obtained by astigmatic imaging with strength described in the main text. (a) Various strengths of astigmatic imaging [3]. We assume the wavefunction $\psi(x_F, y_F)$ is multiplied by a phase factor $\exp[i\varphi(x_F, y_F)]$ before being focused by a lens to a camera placed at the image plane. Here $\varphi(x_F, y_F) = A_{\text{astig.}}\sqrt{6}(x_F^2 - y_F^2)$ with the strength $A_{\text{astig.}}$ varied as indicated by the colorbar. (b) Imaging with various strengths of the self-bending PSF [4]. Again we assume the wavefunction $\psi(x_F, y_F)$ is multiplied by a phase factor $\exp[i\varphi(x_F, y_F)]$ before being focused by a lens to a camera placed at the image plane, but now with $\varphi(x_F, y_F) = A_{\text{SB}}[(x_F + y_F)^3 + (x_F - y_F)^3]$ and $A_{\text{SB}}$ indicated by the colorbar. (c) Bi-plane imaging [5]. The wavefunction is split by a 50/50 beam splitter, then an equal and opposite amount of defocus is introduced into each of the two output channels before focusing with two lenses onto two cameras placed at the image planes. Mathematically: $\psi(x_F, y_F) \rightarrow \psi\left(x_F^+, y_F^+\right) \exp\left[ik\Delta z\sqrt{1 - \left(r_F^+\right)^2}\right]/\sqrt{2} + \psi\left(x_F^-, y_F^-\right) \exp\left[-ik\Delta z\sqrt{1 - \left(r_F^-\right)^2}\right]/\sqrt{2}$. The parameter $\Delta z$ is varied as indicated by the colorbar.

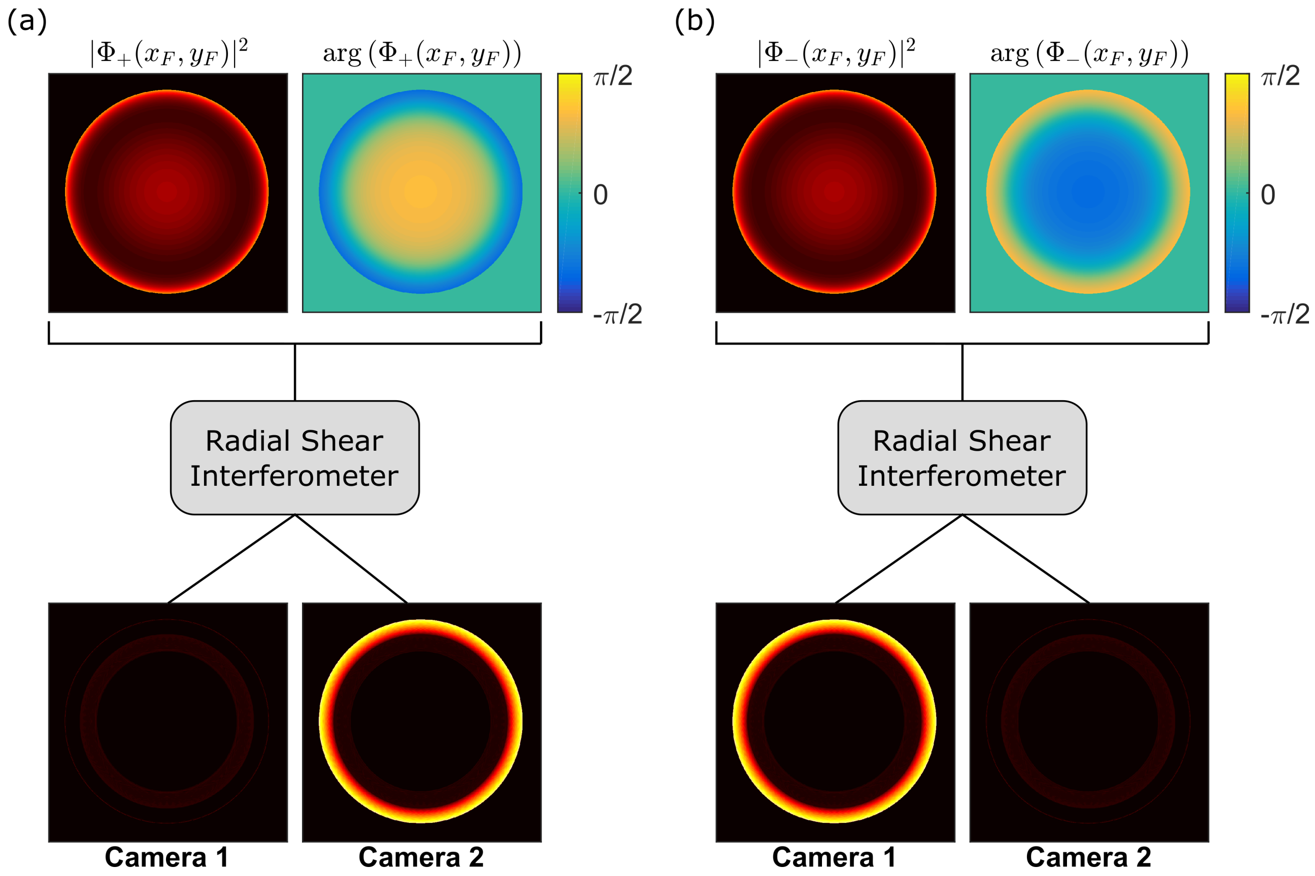


FIG. S3. Schematic depicting how the radial shear interferometer relates to projections onto the eigenstates of $\mathcal{L}_z$ for the single objective case. These eigenstates $|\Phi_+\rangle$ and $|\Phi_-\rangle$ and their associated classical wavefunctions $\Phi_+(x_F, y_F)$ and $\Phi_-(x_F, y_F)$ are described in Section III. (a) Top: intensity and phase associated with $\Phi_+$. Inputting $\Phi_+$ to the radial shear interferometer results in an output (bottom) in which most of the light is incident on Camera 2 and relatively little on Camera 1. Thus the interferometer approximates a projection onto the state $|\Phi_+\rangle$. (b) Top: intensity and phase associated with $\Phi_-$. Note the same intensity and opposite phase as in (a). Inputting $\Phi_-$ to the radial shear interferometer results in an output (bottom) in which most of the light is incident on Camera 1 and relatively little on Camera 2. Thus the interferometer approximates an orthogonal projection onto the state $|\Phi_-\rangle$.

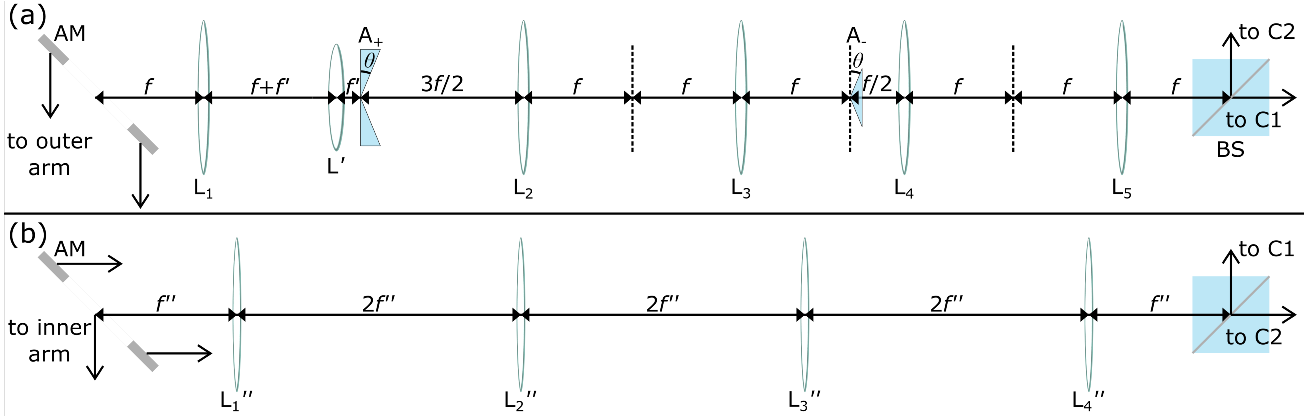


FIG. S4. Schematic of radial shear interferometer showing unfolded arms of the interferometer and exact distances between optical elements. (a) Unfolded inner arm including annular mirror (AM), lenses $L_i$ with focal length $f = 200$ mm, lens $L'$ with focal length $f' = 44$ mm, positive-phase axicon ($A_+$), negative-phase axicon ($A_-$), and beam splitter (BS). (b) Unfolded outer arm including lenses $L''_j$ with focal length $f = 261$ mm.

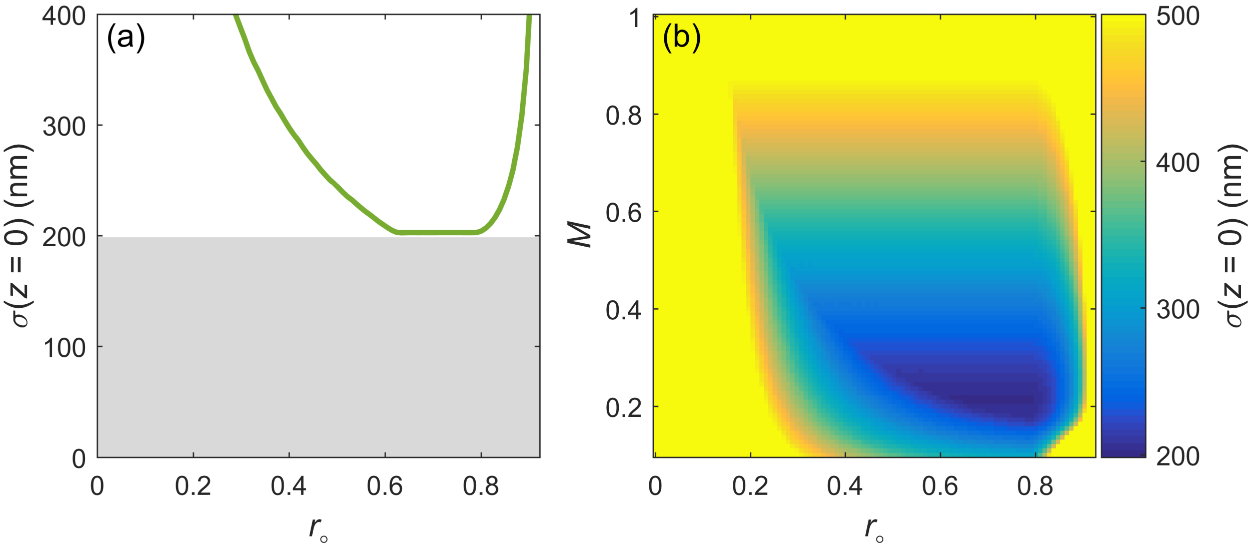


FIG. S5. Photon-normalized CRB of $z$ precision for radial shear interferometer as a function of the parameters $r_\circ$ and $M$. (a) One-dimensional slice of the function for fixed $M$ and variable $r_\circ$ (green line). Gray box again indicates region below QCRB. (b) Two-dimensional depiction of the function. Minimum of the colormap corresponds to the QCRB. The maximum value of the colormap is set to match the dynamic range of the interesting region, at the expense of saturating the outer portion of the image.

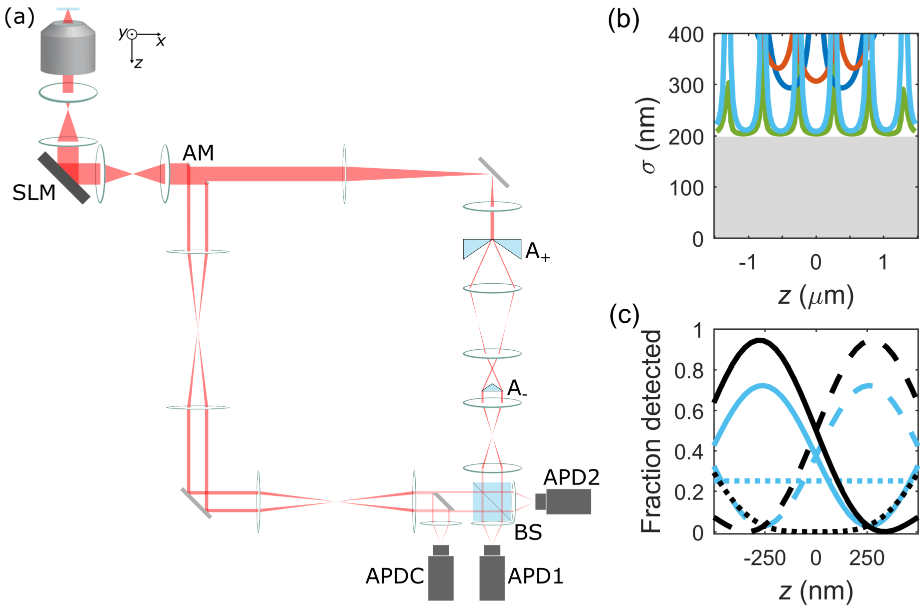


FIG. S6. A variation of the radial shear interferometer in which three point detectors, e.g., avalanche photodiodes (APD), are used instead of two cameras. (a) Schematic of setup showing the output ports of the beam splitter focused onto detectors APD1 and APD2. A mirror of radius $(\mathrm{NA}/n - Mr_\circ)$ is added to the outer arm just before the beam splitter in order to pick off the light that has no counterpart in the inner arm. This light is detected on a complementary detector APDC. (b) Photon-normalized CRB of $z$ precision for single-objective case. Gray box indicates region below QCRB. Lines indicate standard PSF (blue), astigmatism of the same strength described in the main text (red), the two-camera radial shear interferometer (green), and the three-APD radial shear interferometer depicted in (a) (cyan). The minimum of the three-APD variant is approximately $1.05 \times \sigma_z^{(\mathrm{QCRB})}$, slightly worse than the minimum of the two-camera version of approximately $1.03 \times \sigma_z^{(\mathrm{QCRB})}$. (c) Comparison of the three detection channels of the three-APD radial shear interferometer (cyan) and the optimal measurement of projection onto the eigenstates of $\mathcal{L}_z$ (black; see Section III). For cyan lines, solid is the expected fraction of photons detected on APD1, dashed is that for APD2, and dotted is that for APDC. For black lines, solid indicates $|\langle\Phi_-|\psi\rangle|^2$, dashed is $|\langle\Phi_+|\psi\rangle|^2$, and dotted is $1 - |\langle\Phi_-|\psi\rangle|^2 - |\langle\Phi_+|\psi\rangle|^2$. Here $|\Phi_+\rangle$ and $|\Phi_-\rangle$ are chosen to resolve $\mathcal{L}_z$ in a region near $z = 0$, as explained in Section III.

## II. DERIVATION OF SINGLE-OBJECTIVE QCRB

Here we derive the QFI and QCRB for localization with single-objective collection. As discussed in the main text and derived more explicitly in Ref. [6], for thermal light of sufficient weakness (which permits the assumption of Poisson photon statistics), the dominant contribution to the QFI comes from the one-photon term. Thus to derive the applicable QFI we can compute that corresponding to the one-photon state given by $\rho = |\psi\rangle\langle\psi|$, with $|\psi\rangle$ defined by:

$$|\psi\rangle = \iint \mathrm{d}A_F \psi\left(x_F, y_F; \mathbf{x}\right)|x_F, y_F\rangle\,, \tag{S1}$$

and

$$\psi\left(x_F, y_F; \mathbf{x}\right) = \mathcal{A}\left(1 - r_F^2\right)^{-1/4} \mathrm{Circ}\left(\frac{n r_F}{NA}\right) \exp\left[ik\left(x x_F + y y_F + z\sqrt{1 - r_F^2}\right)\right]. \tag{S2}$$

Since $\rho = |\psi\rangle\langle\psi|$ describes a pure state, we could save some algebra and compute the QFI directly from:

$$\mathcal{K}_{ij} = 4\left[\mathrm{Re}\,\langle\partial_i\psi|\partial_j\psi\rangle + \langle\psi|\partial_i\psi\rangle\langle\psi|\partial_j\psi\rangle\right], \tag{S3}$$

which is proportional to the Fubini-Study metric [7]. We instead choose to first find expressions for the symmetric logarithmic derivative operators (SLDs) and proceed as described in the main text, as the SLDs will be referenced in the next Section. The SLDs are given implicitly by the relations:

$$\partial_x\rho = \frac{1}{2}\left(\mathcal{L}_x\rho + \rho\mathcal{L}_x\right), \tag{S4a}$$

$$\partial_y\rho = \frac{1}{2}\left(\mathcal{L}_y\rho + \rho\mathcal{L}_y\right), \tag{S4b}$$

$$\partial_z\rho = \frac{1}{2}\left(\mathcal{L}_z\rho + \rho\mathcal{L}_z\right), \tag{S4c}$$

where $\partial_{x_i}\rho = |\partial_{x_i}\psi\rangle\langle\psi| + |\psi\rangle\langle\partial_{x_i}\psi|$ for each $i$.

Let $\{|l\rangle\}$ be the set of eigenstates of $\rho$ with corresponding eigenvalues $\{D_l\}$. In this basis each $\mathcal{L}_{x_i} \in \{\mathcal{L}_x, \mathcal{L}_y, \mathcal{L}_z\}$ can be defined explicitly [6]:

$$\mathcal{L}_{x_i} = \sum_{l,l';D_l+D_{l'}\neq 0} \frac{2}{D_l + D_{l'}}\langle l|\partial_{x_i}\rho|l'\rangle\,|l\rangle\langle l'|\,. \tag{S5}$$

Clearly $|\psi\rangle$ is one eigenstate of $\rho$ with eigenvalue 1. All other eigenstates of $\rho$ have eigenvalue 0. States $|l\rangle$ for which $\rho\,|l\rangle = \mathbf{0}$ contribute to the sum in Eq. (S5) if $(\partial_{x_i}\rho)\,|l\rangle \neq \mathbf{0}$ for some $i$. Consider the state vectors:

$$|\partial_x\psi\rangle = \iint \mathrm{d}A_F (ikx_F)\psi\left(x_F, y_F; \mathbf{x}\right)|x_F, y_F\rangle\,, \tag{S6a}$$

$$|\partial_y\psi\rangle = \iint \mathrm{d}A_F (iky_F)\psi\left(x_F, y_F; \mathbf{x}\right)|x_F, y_F\rangle\,, \tag{S6b}$$

$$|\partial_z\psi\rangle = \iint \mathrm{d}A_F \left(ik\sqrt{1-r_F^2}\right)\psi\left(x_F, y_F; \mathbf{x}\right)|x_F, y_F\rangle\,. \tag{S6c}$$

We seek an orthonormal basis $\mathscr{B}$ for the Hilbert space spanned by $|\psi\rangle$, $|\partial_x\psi\rangle$, $|\partial_y\psi\rangle$, and $|\partial_z\psi\rangle$. Note that elements of $\{|\psi\rangle\,, |\partial_x\psi\rangle\,, |\partial_y\psi\rangle\}$ are mutually orthogonal, as the relevant overlap integrals each have integrands that are odd functions of $x_F$ and/or $y_F$. The latter two need only to be normalized. We evaluate the norm of $|\partial_x\psi\rangle$:

$$\begin{aligned}\langle\partial_x\psi|\partial_x\psi\rangle &= k^2\mathcal{A}^2 \iint \mathrm{d}A_F \frac{x_F^2}{\sqrt{1-r_F^2}}\mathrm{Circ}\left(\frac{nr_F}{\mathrm{NA}}\right)\\ &= k^2\mathcal{A}^2 \int_0^{\mathrm{NA}/n} r_F \mathrm{d}r_F \int_0^{2\pi} \mathrm{d}\varphi_F \frac{r_F^2\cos^2\varphi_F}{\sqrt{1-r_F^2}}\\ &= \frac{\pi k^2\mathcal{A}^2}{3}\left[2 - \left(2 + (\mathrm{NA}/n)^2\right)\sqrt{1-(\mathrm{NA}/n)^2}\right].\end{aligned} \tag{S7}$$

One can show that $\langle\partial_y\psi|\partial_y\psi\rangle = \langle\partial_x\psi|\partial_x\psi\rangle$. Define

$$C_{xy} = \frac{1}{\sqrt{\langle\partial_x\psi|\partial_x\psi\rangle}} = \frac{1}{\sqrt{\langle\partial_y\psi|\partial_y\psi\rangle}}, \tag{S8}$$

and

$$|\psi_x\rangle = C_{xy}\,|\partial_x\psi\rangle\,, \tag{S9a}$$

$$|\psi_y\rangle = C_{xy}\,|\partial_y\psi\rangle\,. \tag{S9b}$$

Now $\{|\psi\rangle\,, |\psi_x\rangle\,, |\psi_y\rangle\}$ is orthonormal. One more basis vector must be added to construct $\mathscr{B}$ such that it includes $|\partial_z\psi\rangle$ in its span. We have $\langle\psi_x|\partial_z\psi\rangle = \langle\psi_y|\partial_z\psi\rangle = 0$ since again these overlap integrals have integrands that are odd functions of $x_F$ and $y_F$, respectively. However, $\gamma \equiv \langle\psi|\partial_z\psi\rangle \neq 0$. In fact we can evaluate $\gamma$ analytically:

$$\gamma = ik\mathcal{A}^2 \iint \mathrm{d}A_F \mathrm{Circ}\left(\frac{nr_F}{\mathrm{NA}}\right)$$
$$= ik\mathcal{A}^2 \pi (\mathrm{NA}/n)^2. \tag{S10}$$

Letting

$$C_z = \frac{1}{\sqrt{\langle \partial_z \psi | \partial_z \psi \rangle}}$$
$$= \frac{\sqrt{3}}{k\mathcal{A}\sqrt{2\pi}} \left[1 - \left(1 - (\mathrm{NA}/n)^2\right)^{3/2}\right]^{-1/2}, \tag{S11}$$

we can proceed by the Gram-Schmidt algorithm to obtain:

$$|\psi_z\rangle = \frac{|\partial_z \psi\rangle - \gamma |\psi\rangle}{\sqrt{C_z^{-2} - |\gamma|^2}}. \tag{S12}$$

The result is the orthonormal basis $\mathscr{B} = \{|\psi\rangle, |\psi_x\rangle, |\psi_y\rangle, |\psi_z\rangle\}$. The operators of the LHS of Eq. (S4) can be expressed:

$$\partial_x \rho = \frac{1}{C_{xy}} \Big( |\psi\rangle \langle \psi_x| + |\psi_x\rangle \langle \psi| \Big), \tag{S13a}$$
$$\partial_y \rho = \frac{1}{C_{xy}} \Big( |\psi\rangle \langle \psi_y| + |\psi_y\rangle \langle \psi| \Big), \tag{S13b}$$
$$\partial_z \rho = \sqrt{C_z^{-2} - |\gamma|^2} \Big( |\psi\rangle \langle \psi_z| + |\psi_z\rangle \langle \psi| \Big). \tag{S13c}$$

The SLDs can now be computed directly from Eqs. (S5) and (S13) to give:

$$\mathcal{L}_x = \frac{2}{C_{xy}} \Big( |\psi\rangle \langle \psi_x| + |\psi_x\rangle \langle \psi| \Big), \tag{S14a}$$
$$\mathcal{L}_y = \frac{2}{C_{xy}} \Big( |\psi\rangle \langle \psi_y| + |\psi_y\rangle \langle \psi| \Big), \tag{S14b}$$
$$\mathcal{L}_z = 2\sqrt{C_z^{-2} - |\gamma|^2} \Big( |\psi\rangle \langle \psi_z| + |\psi_z\rangle \langle \psi| \Big). \tag{S14c}$$

The elements of the quantum Fisher information matrix $\mathcal{K}$ can be computed according to:

$$\mathcal{K}_{ij} = \frac{1}{2} \mathrm{Re\ Tr}\ \rho \left( \mathcal{L}_{x_i} \mathcal{L}_{x_j} + \mathcal{L}_{x_j} \mathcal{L}_{x_i} \right), \tag{S15}$$

yielding the result:

$$\mathcal{K} = 4 \begin{pmatrix} C_{xy}^{-2} & 0 & 0 \\ 0 & C_{xy}^{-2} & 0 \\ 0 & 0 & C_z^{-2} - |\gamma|^2 \end{pmatrix}. \tag{S16}$$

The quantum Cramér-Rao bounds for each dimension are given simply by the inverse square roots of the diagonal elements in Eq. (S16):

$$\sigma_x^{(\mathrm{QCRB})} = C_{xy}/2, \tag{S17a}$$

$$\sigma_y^{(\mathrm{QCRB})} = C_{xy}/2, \tag{S17b}$$

$$\sigma_z^{(\mathrm{QCRB})} = \left(C_z^{-2} - |\gamma|^2\right)^{-1/2}/2. \tag{S17c}$$

## III. ON THE EIGENSTATES OF THE SINGLE-OBJECTIVE $\mathcal{L}_z$

In this work we present a variant of a radial shear interferometer that numerically approaches the QCRB with respect to $z$ estimation in the case of single-objective detection. It has been noted elsewhere [8] that a sufficient condition for saturating the QCRB is for a measurement to produce projections onto the eigenstates of the relevant symmetric logarithmic derivative, in this case $\mathcal{L}_z$. Here we describe the relation between the radial shear interferometer and such a projection measurement.

In Section II we show that $\mathcal{L}_z$ can be expressed:

$$\mathcal{L}_z = 2\sqrt{C_z^{-2} - |\gamma|^2}\left(|\psi\rangle\langle\psi_z| + |\psi_z\rangle\langle\psi|\right), \tag{S18}$$

with $C_z$, $\gamma$, and $|\psi_z\rangle$ defined in Eqs. (S10), (S11), and (S12), respectively. $\mathcal{L}_z$ has eigenstates $|\Phi_+\rangle$ and $|\Phi_-\rangle$ defined by:

$$|\Phi_+\rangle = \frac{1}{\sqrt{2}}\left(|\psi\rangle + |\psi_z\rangle\right), \tag{S19a}$$

$$|\Phi_-\rangle = \frac{1}{\sqrt{2}}\left(|\psi\rangle - |\psi_z\rangle\right). \tag{S19b}$$

With a little algebra we can write:

$$|\Phi_+\rangle = \iint \mathrm{d}A_F \Phi_+\left(x_F, y_F\right)|x_F, y_F\rangle, \tag{S20a}$$

$$|\Phi_-\rangle = \iint \mathrm{d}A_F \Phi_-\left(x_F, y_F\right)|x_F, y_F\rangle, \tag{S20b}$$

where the classical wavefunctions $\Phi_+(x_F, y_F)$ and $\Phi_-(x_F, y_F)$ are defined by:

$$\Phi_+(x_F, y_F) = \frac{1}{\sqrt{2}}\left(1 + \frac{ik\sqrt{1-r_F^2} - \gamma}{\sqrt{C_Z^{-2} - |\gamma|^2}}\right)\psi(x_F, y_F), \tag{S21a}$$

$$\Phi_-(x_F, y_F) = \frac{1}{\sqrt{2}}\left(1 - \frac{ik\sqrt{1-r_F^2} - \gamma}{\sqrt{C_Z^{-2} - |\gamma|^2}}\right)\psi(x_F, y_F). \tag{S21b}$$

Note that since $\psi(x_F, y_F)$ depends implicitly on $z$, so too do $\Phi_+(x_F, y_F)$ and $\Phi_-(x_F, y_F)$. A measurement that produces the desired projections for a particular choice of $z$ is only guaranteed to achieve the QCRB in a region near that $z$, a microcosm of a more general phenomenon in quantum statistical estimation in which the optimality of the measurement often depends on the state itself [9]. Figure S3 depicts both the intensity and phase functions associated with $\Phi_+(x_F, y_F)$ and $\Phi_-(x_F, y_F)$ for $z = 0$. To determine how the operation of the radial shear interferometer compares to the projection operators $\{|\Phi_+\rangle\langle\Phi_+|, |\Phi_-\rangle\langle\Phi_-|\}$ we compute the diffraction integrals described in Section IV with both $\Phi_+(x_F, y_F)$ and $\Phi_-(x_F, y_F)$ as inputs. The results are illustrated in Fig. S3. We find that when $|\Phi_+\rangle$ is input to our interferometer the vast majority of the light is shunted to detector 2, while inputting $|\Phi_-\rangle$ results in the majority of signal falling on detector 1. In effect we see that our radial shear interferometer approximates projection on the eigenstates of $\mathcal{L}_z$. The fact that the approximation is not exact is consistent with the fact that the CRB attained by the interferometer as presently parameterized is actually slightly greater than the QCRB. As mentioned elsewhere in this work, the approximation can be further improved by adding arms to the interferometer that employ the unused inner ring of light.

## IV. DETAILS FOR RADIAL SHEAR INTERFEROMETER

In this section we describe the radial shear interferometer setup in greater detail, giving exact values of parameters and describing the diffraction integrals computed in simulating the measurement. Figure S4 shows schematics of the inner and outer arms of the interferometer, unfolded for clarity and with exact distances labeled.

In the main text we define the wavefunction at the Fourier plane at the back aperture of

the objective lens by

$$\psi(x_F, y_F) = \mathcal{A}\left(1 - r_F^2\right)^{-1/4} \mathrm{Circ}\left(\frac{n r_F}{\mathrm{NA}}\right) \exp\left[ik\left(x x_F + y y_F + z\sqrt{1 - r_F^2}\right)\right], \tag{S22}$$

where the spatial coordinates $x_F$, $y_F$, and $r_F = \sqrt{x_F^2 + y_F^2}$ are scaled such that the support of $\psi(x_F, y_F)$ is $r_F \leq \mathrm{NA}/n$. As discussed in the main text, what we mean by this formalism is that the light is in a statistical state with normalized Fourier-plane mutual coherence function $g(x_F, y_F, x'_F, y'_F) = \psi(x_F, y_F)\psi^*(x'_F, y'_F)$. We can obtain the normalized mutual coherence function at the detectors by propagating $\psi(x_F, y_F)$ to the detector planes via the ordinary rules of linear optics, then taking the analogous outer product.

Invoking the Abbe sine condition, we can relate the scaled coordinates in Eq. (S22) to unscaled coordinates $\tilde{x}_F$, $\tilde{y}_F$, and $\tilde{r}_F$ via:

$$\tilde{x}_F = \frac{n f_{\mathrm{TL}}}{\sqrt{M_{\mathrm{sys}}^2 - \mathrm{NA}^2}} x_F, \tag{S23a}$$

$$\tilde{y}_F = \frac{n f_{\mathrm{TL}}}{\sqrt{M_{\mathrm{sys}}^2 - \mathrm{NA}^2}} y_F, \tag{S23b}$$

$$\tilde{r}_F = \frac{n f_{\mathrm{TL}}}{\sqrt{M_{\mathrm{sys}}^2 - \mathrm{NA}^2}} r_F, \tag{S23c}$$

where $f_{\mathrm{TL}}$ is the focal length of the tube lens and $M_{\mathrm{sys}}$ is the magnification of the objective-tube lens unit (i.e., the magnification written on the objective casing, assuming the company-intended tube lens is used). For our purposes we assume $M_{\mathrm{sys}} = 100$ and $f_{\mathrm{TL}} = 180$ mm, the latter of which is the standard for Olympus microscopes. For such a system magnification we can approximate $\sqrt{M_{\mathrm{sys}}^2 - \mathrm{NA}^2} \approx M_{\mathrm{sys}}$ such that the unscaled coordinates can be redefined more simply:

$$\tilde{x}_F = \frac{n f_{\mathrm{TL}}}{M_{\mathrm{sys}}} x_F, \tag{S24a}$$

$$\tilde{y}_F = \frac{n f_{\mathrm{TL}}}{M_{\mathrm{sys}}} y_F, \tag{S24b}$$

$$\tilde{r}_F = \frac{n f_{\mathrm{TL}}}{M_{\mathrm{sys}}} r_F. \tag{S24c}$$

In the main text we describe imparting a small amount of defocus at a conjugate Fourier plane (i.e., using an SLM) before the annular mirror in order to compensate for defocus accrued downstream. A defocus equivalent to $\Delta z = 73$ nm approximately achieves this goal

for the arrangement depicted in Fig. S4. In practice $\Delta z$ can be modulated to feedback on the position of a tracked emitter. The wavefunction at the conjugate Fourier plane just before the annular mirror, as a function of unscaled coordinates, can then be defined:

$$\tilde{\psi}\left(\tilde{x}_F, \tilde{y}_F\right) = \left(\frac{M_{\text{sys}}}{n f_{\text{TL}}}\right) \psi\left(\frac{M_{\text{sys}}}{n f_{\text{TL}}}\tilde{x}_F, \frac{M_{\text{sys}}}{n f_{\text{TL}}}\tilde{y}_F\right) \exp\left[ik\Delta z\sqrt{1-\left(\frac{M_{\text{sys}}}{n f_{\text{TL}}}\tilde{r}_F\right)^2}\right], \tag{S25}$$

where the prefactor ensures $\iint \mathrm{d}\tilde{x}_F \mathrm{d}\tilde{y}_F |\tilde{\psi}\left(\tilde{x}_F, \tilde{y}_F\right)|^2 = 1$.

We will now trace the transformation of $\tilde{\psi}\left(\tilde{x}_F, \tilde{y}_F\right)$ through the inner arm of the interferometer [Fig. S4(a)]. As described in the main text, the inner radius of the annular mirror (in scaled units) is $r_\circ = 0.6326$, such that the wavefunction in the inner arm just after the annular mirror is:

$$\psi^{(\text{i})}\left(x^{(\text{i})}, y^{(\text{i})}\right) = \tilde{\psi}\left(x^{(\text{i})}, y^{(\text{i})}\right) \text{Circ}\left(\frac{M_{\text{sys}}}{n f_{\text{TL}} r_\circ} r^{(\text{i})}\right), \tag{S26}$$

where $x^{(\text{i})}$, $y^{(\text{i})}$, and $r^{(\text{i})} = \sqrt{(x^{(\text{i})})^2 + (y^{(\text{i})})^2}$ are the coordinates defined in this plane.

The lenses labeled $\text{L}_i$ for $i \in \{1, 2, 3, 4, 5\}$ in Fig. S4(a) have a common focal length of $f = 200$ mm. A second type of lens labeled L′ in Fig. S4(a) has a shorter focal length of $f' = 44$ mm, chosen such that the the wavefunction at the back focal plane of L′ is demagnified by a factor $M = f'/f = 0.22$. At this plane, just before the first axicon lens ($\text{A}_+$), the wavefunction is:

$$\psi^{(\text{ii})}\left(x^{(\text{ii})}, y^{(\text{ii})}\right) = \frac{1}{M}\psi^{(\text{i})}\left(-\frac{x^{(\text{ii})}}{M}, -\frac{y^{(\text{ii})}}{M}\right). \tag{S27}$$

As described in the main text, the axicon $\text{A}_+$ imparts a phase delay proportional to distance from the optical axis. We heuristically choose a proportionality constant such that the wavefunction just after $\text{A}_+$ is given by:

$$\psi^{(\text{iii})}\left(x^{(\text{iii})}, y^{(\text{iii})}\right) = \psi^{(\text{ii})}\left(x^{(\text{iii})}, y^{(\text{iii})}\right) \exp\left[\frac{680 i M_{\text{sys}}}{n f_{\text{TL}}} r^{(\text{iii})}\right]. \tag{S28}$$

As an aside, we here consider the implication of Eq. (S28) on the inclination angle $\theta$ labeled in Fig. S4(a). Assuming the axicon is made of glass with index of refraction $n = 1.518$ (i.e., equal to that of the objective immersion oil), one can deduce from geometry:

$$\theta = \arctan\left(\frac{680\lambda M_{\text{sys}}}{2\pi(n-1) n f_{\text{TL}}}\right) \approx 2.9°. \tag{S29}$$

Next we seek an expression for the wavefunction after propagation from the axicon $A_+$ to the back focal plane of lens $L_2$. This can be obtained as a scaled Fourier transform multiplied by a quadratic phase factor [10]:

$$\psi^{(\mathrm{iv})}\left(x^{(\mathrm{iv})}, y^{(\mathrm{iv})}\right) = \frac{\exp\left(-\frac{i\pi}{2\lambda f}\left[(x^{(\mathrm{iv})})^2 + (y^{(\mathrm{iv})})^2\right]\right)}{i\lambda f} \times \iint \mathrm{d}x^{(\mathrm{iii})}\mathrm{d}y^{(\mathrm{iii})}\psi^{(\mathrm{iii})}\left(x^{(\mathrm{iii})}, y^{(\mathrm{iii})}\right)\exp\left(-\frac{2\pi i}{\lambda f}\left[x^{(\mathrm{iii})}x^{(\mathrm{iv})} + y^{(\mathrm{iii})}y^{(\mathrm{iv})}\right]\right). \tag{S30}$$

In practice we computed Eq. (S30) and subsequent diffraction integrals numerically via appropriate application of the MATLAB function fft2. Propagation to the back focal plane of lens $L_3$, just before the axicon $A_-$, gives the wavefunction:

$$\psi^{(\mathrm{v})}\left(x^{(\mathrm{v})}, y^{(\mathrm{v})}\right) = \frac{1}{i\lambda f}\iint \mathrm{d}x^{(\mathrm{iv})}\mathrm{d}y^{(\mathrm{iv})}\psi^{(\mathrm{iv})}\left(x^{(\mathrm{iv})}, y^{(\mathrm{iv})}\right)\exp\left(-\frac{2\pi i}{\lambda f}\left[x^{(\mathrm{iv})}x^{(\mathrm{v})} + y^{(\mathrm{iv})}y^{(\mathrm{v})}\right]\right). \tag{S31}$$

The axicon $A_-$ imparts a phase delay of opposite sign to that of $A_+$ such that just after $A_-$ we have:

$$\psi^{(\mathrm{vi})}\left(x^{(\mathrm{vi})}, y^{(\mathrm{vi})}\right) = \psi^{(\mathrm{v})}\left(x^{(\mathrm{vi})}, y^{(\mathrm{vi})}\right)\exp\left[-\frac{680 i M_{\mathrm{sys}}}{n f_{\mathrm{TL}}} r^{(\mathrm{vi})}\right]. \tag{S32}$$

At the back focal plane of lens $L_4$ we have:

$$\psi^{(\mathrm{vii})}\left(x^{(\mathrm{vii})}, y^{(\mathrm{vii})}\right) = \frac{\exp\left(\frac{i\pi}{2\lambda f}\left[(x^{(\mathrm{vii})})^2 + (y^{(\mathrm{vii})})^2\right]\right)}{i\lambda f} \times \iint \mathrm{d}x^{(\mathrm{vi})}\mathrm{d}y^{(\mathrm{vi})}\psi^{(\mathrm{vi})}\left(x^{(\mathrm{vi})}, y^{(\mathrm{vi})}\right)\exp\left(-\frac{2\pi i}{\lambda f}\left[x^{(\mathrm{vi})}x^{(\mathrm{vii})} + y^{(\mathrm{vi})}y^{(\mathrm{vii})}\right]\right), \tag{S33}$$

and at the back focal plane of lens $L_5$:

$$\psi^{(\mathrm{viii})}\left(x^{(\mathrm{viii})}, y^{(\mathrm{viii})}\right) = \frac{1}{i\lambda f}\iint \mathrm{d}x^{(\mathrm{vii})}\mathrm{d}y^{(\mathrm{vii})}\psi^{(\mathrm{vii})}\left(x^{(\mathrm{vii})}, y^{(\mathrm{vii})}\right) \times \exp\left(-\frac{2\pi i}{\lambda f}\left[x^{(\mathrm{vii})}x^{(\mathrm{viii})} + y^{(\mathrm{vii})}y^{(\mathrm{viii})}\right]\right). \tag{S34}$$

Next we consider the transformations in the outer arm of the interferometer [Fig. S4(b)]. Just after the annular mirror the wavefunction in this arm is given simply by:

$$\psi^{(\mathrm{o})}\left(x^{(\mathrm{o})}, y^{(\mathrm{o})}\right) = \tilde{\psi}\left(-x^{(\mathrm{o})}, y^{(\mathrm{o})}\right) - \psi^{(\mathrm{i})}\left(-x^{(\mathrm{o})}, y^{(\mathrm{o})}\right). \tag{S35}$$

Each lens $L''_j$ for $j \in \{1,2,3,4\}$ in the outer arm has focal length $f'' = 261$ mm, chosen such that the total distance from annular mirror to beam splitter is the same as that in the inner arm (2.088 m). The lenses $L''_j$ are arranged such that they form two sequential telescopes of unit magnification, effectively relaying $\psi^{(\mathrm{o})}$ to the beam splitter plane unchanged.

Finally, just after the beam splitter the wavefunctions in each of the output ports are given by:

$$\psi^{(\mathrm{C1})}\left(x^{(\mathrm{C1})}, y^{(\mathrm{C1})}\right) = \frac{1}{\sqrt{2}}\left[\psi^{(\mathrm{viii})}\left(x^{(\mathrm{C1})}, y^{(\mathrm{C1})}\right) + i\psi^{(\mathrm{o})}\left(-x^{(\mathrm{C1})}, y^{(\mathrm{C1})}\right)\right], \tag{S36a}$$

$$\psi^{(\mathrm{C2})}\left(x^{(\mathrm{C2})}, y^{(\mathrm{C2})}\right) = \frac{1}{\sqrt{2}}\left[i\psi^{(\mathrm{viii})}\left(-x^{(\mathrm{C2})}, y^{(\mathrm{C2})}\right) + \psi^{(\mathrm{o})}\left(x^{(\mathrm{C2})}, y^{(\mathrm{C2})}\right)\right]. \tag{S36b}$$

## V. DERIVATION OF DUAL-OBJECTIVE QCRB

Here we will derive the QFI and QCRB for localization with dual-objective collection. Again, as justified in the main text and in Section II of the Supplemental Material, we can begin our calculation by considering the state $\rho = |\psi\rangle\langle\psi|$. However now the single-photon state $|\psi\rangle$ is distributed among coordinates localized to the back apertures of both objectives $a$ and $b$ [refer to Fig. 3(b) of the main text]:

$$|\psi\rangle = \frac{1}{\sqrt{2}}\left(|\psi^{(a)}\rangle + |\psi^{(b)}\rangle\right), \tag{S37}$$

where

$$|\psi^{(a)}\rangle = \iint \mathrm{d}A_F^{(a)} \psi\left(x_F^{(a)}, y_F^{(a)}; [x,y,z]^{\mathrm{T}}\right)\left|x_F^{(a)}, y_F^{(a)}\right\rangle, \tag{S38}$$

and

$$|\psi^{(b)}\rangle = \iint \mathrm{d}A_F^{(b)} \psi\left(x_F^{(b)}, y_F^{(b)}; [-x,y,-z]^{\mathrm{T}}\right)\left|x_F^{(b)}, y_F^{(b)}\right\rangle. \tag{S39}$$

Here

$$\psi\left(x_F^{(a)}, y_F^{(a)}; [x,y,z]^{\mathrm{T}}\right) = \mathcal{A}\left(1 - \left(r_F^{(a)}\right)^2\right)^{-1/4} \mathrm{Circ}\left(\frac{n r_F^{(a)}}{NA}\right) \times \exp\left[ik\left(x x_F^{(a)} + y y_F^{(a)} + z\sqrt{1 - \left(r_F^{(a)}\right)^2}\right)\right], \tag{S40}$$

and

$$\psi\left(x_F^{(b)}, y_F^{(b)}; [-x, y, -z]^{\mathrm{T}}\right) = \mathcal{A}\left(1 - \left(r_F^{(b)}\right)^2\right)^{-1/4} \mathrm{Circ}\left(\frac{n r_F^{(b)}}{NA}\right) \times \exp\left[ik\left(-x x_F^{(b)} + y y_F^{(b)} - z\sqrt{1 - \left(r_F^{(b)}\right)^2}\right)\right]. \quad \text{(S41)}$$

In this case, rather than proceeding by finding expressions for the SLDs, we conserve lines of algebra and compute directly from Eq. (S3). The states $|\partial_x\psi\rangle$, $|\partial_y\psi\rangle$, and $|\partial_z\psi\rangle$ are now given by:

$$|\partial_x\psi\rangle = \frac{ik}{\sqrt{2}}\left[\iint \mathrm{d}A_F^{(a)} x_F^{(a)} \psi\left(x_F^{(a)}, y_F^{(a)}; [x, y, z]^{\mathrm{T}}\right)\left|x_F^{(a)}, y_F^{(a)}\right\rangle - \iint \mathrm{d}A_F^{(b)} x_F^{(b)} \psi\left(x_F^{(b)}, y_F^{(b)}; [-x, y, -z]^{\mathrm{T}}\right)\left|x_F^{(b)}, y_F^{(b)}\right\rangle\right], \quad \text{(S42a)}$$

$$|\partial_y\psi\rangle = \frac{ik}{\sqrt{2}}\left[\iint \mathrm{d}A_F^{(a)} y_F^{(a)} \psi\left(x_F^{(a)}, y_F^{(a)}; [x, y, z]^{\mathrm{T}}\right)\left|x_F^{(a)}, y_F^{(a)}\right\rangle + \iint \mathrm{d}A_F^{(b)} y_F^{(b)} \psi\left(x_F^{(b)}, y_F^{(b)}; [-x, y, -z]^{\mathrm{T}}\right)\left|x_F^{(b)}, y_F^{(b)}\right\rangle\right], \quad \text{(S42b)}$$

$$|\partial_z\psi\rangle = \frac{ik}{\sqrt{2}}\left[\iint \mathrm{d}A_F^{(a)} \sqrt{1 - \left(r_F^{(a)}\right)^2} \psi\left(x_F^{(a)}, y_F^{(a)}; [x, y, z]^{\mathrm{T}}\right)\left|x_F^{(a)}, y_F^{(a)}\right\rangle - \iint \mathrm{d}A_F^{(b)} \sqrt{1 - \left(r_F^{(b)}\right)^2} \psi\left(x_F^{(b)}, y_F^{(b)}; [-x, y, -z]^{\mathrm{T}}\right)\left|x_F^{(b)}, y_F^{(b)}\right\rangle\right]. \quad \text{(S42c)}$$

The fact that $\left\langle x_F^{(a)}, y_F^{(a)} \middle| x_F^{(b)}, y_F^{(b)}\right\rangle = 0$ means we can ignore cross terms in evaluating the overlap integrals. As in the single-objective case we can quickly conclude that each of $\{|\psi\rangle, |\partial_x\psi\rangle, |\partial_y\psi\rangle\}$ are mutually orthogonal as the associated integrals all have integrands that are odd functions of $x_F$ and/or $y_F$. Also note that the norms of the derivative states are the same as those of their counterparts in the single-objective case. That is,

$$\langle\partial_x\psi|\partial_x\psi\rangle = 1/C_{xy}^2, \quad \text{(S43a)}$$

$$\langle\partial_y\psi|\partial_y\psi\rangle = 1/C_{xy}^2, \quad \text{(S43b)}$$

$$\langle\partial_z\psi|\partial_z\psi\rangle = 1/C_z^2, \quad \text{(S43c)}$$

where $C_{xy}$ and $C_z$ are exactly as they are defined in Eqs. (S8) and (S11) of Section II. Yet again we have $\langle\psi_x|\partial_z\psi\rangle = \langle\psi_y|\partial_z\psi\rangle = 0$ since these integrals too are odd functions of $x_F$ and

$y_F$, respectively. However, unlike in the single-objective case, we also have $\langle\psi|\partial_z\psi\rangle = 0$:

$$\begin{aligned}\langle\psi|\partial_z\psi\rangle = \frac{k^2}{2}\Bigg[&\iint \mathrm{d}A_F^{(a)}\sqrt{1-\left(r_F^{(a)}\right)^2}\left|\psi\left(x_F^{(a)},y_F^{(a)}\right)\right|^2 \\ &-\iint \mathrm{d}A_F^{(b)}\sqrt{1-\left(r_F^{(b)}\right)^2}\left|\psi\left(x_F^{(b)},y_F^{(b)}\right)\right|^2\Bigg] \\ =\ & 0,\end{aligned} \tag{S44}$$

where in the second line we recognize that the two terms cancel one another. Thus the QFI matrix evaluates to:

$$\mathcal{K} = 4\begin{pmatrix} C_{xy}^{-2} & 0 & 0 \\ 0 & C_{xy}^{-2} & 0 \\ 0 & 0 & C_z^{-2}\end{pmatrix}. \tag{S45}$$

The quantum Cramér-Rao bounds for each dimension are given simply by the inverse square roots of the diagonal elements in Eq. (S45):

$$\sigma_x^{(\mathrm{QCRB})} = C_{xy}/2, \tag{S46a}$$

$$\sigma_y^{(\mathrm{QCRB})} = C_{xy}/2, \tag{S46b}$$

$$\sigma_z^{(\mathrm{QCRB})} = C_z/2. \tag{S46c}$$

## VI. DETAILS OF CALCULATIONS

Cramér-Rao bounds were computed numerically using custom MATLAB software. In all cases we assume quasi-monochromatic emission of vacuum wavelength $\lambda_\circ = 670$ nm, NA $= 1.4$, and a matched sample-immersion index of $n = 1.518$. Propagation through lenses was simulated via properly scaled implementations of the MATLAB function fft2. Image-plane detection schemes were computed such that calculated images were finely sampled with 20-nm $\times$ 20-nm pixels as projected to object space. An exception is the Saddle-Point PSF scheme depicted in Fig. S1; this was more coarsely sampled with 110-nm $\times$ 110-nm pixels. The radial shear interferometer detection scheme was sampled such that the Fourier-plane pixels were approximately of dimensions 0.0027 $\times$ 0.0027 in units of NA$/n$. To facilitate fft calculation the Fourier-plane patterns in this case were zero-padded to a total image size of 2048 $\times$ 2048 pixels.

## VII. REFERENCES

---

[1] Y. Shechtman, S. J. Sahl, A. S. Backer, and W. E. Moerner, Physical Review Letters **113**, 133902 (2014).

[2] Y. Shechtman, L. E. Weiss, A. S. Backer, S. J. Sahl, and W. E. Moerner, Nano Letters **15**, 4194 (2015).

[3] B. Huang, W. Wang, M. Bates, and X. Zhuang, Science **319**, 810 (2008).

[4] S. Jia, J. C. Vaughan, and X. Zhuang, Nature Photonics **8**, 302 (2014).

[5] P. Prabhat, S. Ram, E. S. Ward, and R. J. Ober, IEEE Transactions on Nanobioscience **3**, 237 (2004).

[6] M. Tsang, R. Nair, and X.-M. Lu, Physical Review X **6**, 031033 (2016).

[7] A. Fujiwara and H. Nagaoka, Physics Letters A **201**, 119 (1995).

[8] S. L. Braunstein and C. M. Caves, Physical Review Letters **72**, 3439 (1994).

[9] O. E. Barndorff-Nielsen and R. D. Gill, Journal of Physics A: Mathematical and General **33**, 4481 (2000).

[10] J. W. Goodman, *Introduction to Fourier Optics* (Roberts and Company Publishers, 2005).
